# Supplementary material for: SeeSR: Towards Semantics-Aware Real-World Image Super-Resolution
Source: arXiv:2311.16518 source file (2024-06-04)
Supplement: Supplementary file 1 [file X_suppl.tex]

\clearpage
\setcounter{page}{1}
\maketitlesupplementary

%\section{Supplementary Material}
%\label{sec:suppl}

In this supplementary file, we provide the following materials:
\begin{itemize}
  \item Ablation studies on the proposed LRE strategy and DAPE module (referring to Section 4 in the main paper);
  
  \item Complexity analysis (referring to Section 4 in the main paper);
  
  \item More real-word visual comparisons under scaling factor $4\times$ (referring to Section 4.2 in the main paper).
\end{itemize}

\section{Ablation Study}
We first discuss the effectiveness of the proposed LRE strategy. Then, we discuss the effectiveness of the proposed DAPE module from two aspects: its tagging capability on degraded images and the improvement brought by it on Real-ISR tasks. 

\begin{table}[h] 
\centering
\caption{The Real-ISR performance of our SeeSR model with and without LRE on \textit{DIV2K-Val} and \textit{DrealSR} \cite{drealsr} benchmarks.}
\begin{tabular}{c|cc}
\hline
        & w/o LRE         & w/ LRE          \\ \hline
PSNR $\uparrow$   & 20.58 / 26.55   & 21.04 / 27.90   \\
LPIPS $\downarrow$  & 0.3942 / 0.3952 & 0.3876 / 0.3299 \\
FID $\downarrow$    & 32.53 / 158.04  & 32.79 / 151.88  \\
CLIPIQA & 0.7314 / 0.7248 & 0.6834 / 0.6708 \\ \hline
\end{tabular}
\end{table}

%\noindent
\textbf{Effectiveness of LRE.} We first show the Real-ISR performance of our SeeSR model on the DIV2K-Val and DrealSR datasets with and without the LRE strategy. The results are shown in Table xxx. One can see that the LRE strategy improves the reference-based metrics, including both fidelity and perception based ones, but it weakens the non-reference metrics such as CLIPIQA. This is because the LRE strategy reduces the model’s tendency to generate additional but unfaithful textures by reducing the gap between training and testing (see analysis in Sec. \ref{sec:method_4} of the main paper). Such an over-generation ability can be favorable by metrics like CLIPIQA, but they will introduce visually unpleasant artifacts, as shown in Fig. \ref{fig:elr} of the main paper.

%%%%%% table aba on tag %%%%%%
\begin{table}[h] 
\centering
\caption{Ablation study of DAPE on COCO-Val benchmark \cite{coco} for the tagging task.}
\begin{tabular}{l|lll}
\hline
         & OP $\uparrow$& OR $\uparrow$ & AP $\uparrow$\\ \hline
RAM \cite{2023ram} & 0.7929   & 0.3711   &  52.3   \\
DAPE     & \textbf{0.8940}   &  \textbf{0.3751}  &  \textbf{63.0}   \\ \hline
\end{tabular}
\label{tab:aba_tag}
\end{table}
%%%%%%

\textbf{Improved Tagging Capability.}
In Table \ref{tab:aba_tag}, we present the tagging performance of our DAPE module on the degraded images of COCO-Val benchmark \cite{coco} based on three metrics: overall precision (OP), overall recall (OR), and average precision (AP). AP is the averaged precision calculated on different recall rates, which is similar to the detection metric. OP and OR are defined as:
\begin{equation}
\begin{aligned}
\mathrm{OP} =\frac{\sum_{i} N_{i}^{t}}{\sum_{i} N_{i}^{p}}, && \mathrm{OR} =\frac{\sum_{i} N_{i}^{t}}{\sum_{i} N_{i}^{g}}, 
\end{aligned}
\end{equation}
where $C$ is the number of classes, $N_{i}^{p}$ is the number of images predicted for label $i$, $N_{i}^{t}$ is the number of images correctly predicted for label $i$, and $N_{i}^{g}$ is the number of ground truth images for label $i$.

We evaluated RAM \cite{2023ram} and DAPE with the default threshold. DAPE surpasses RAM in terms of OP and AP by 0.1 and 10.7, respectively. It also maintains superiority in OR, indicating that DAPE achieves significant improvements in tagging accuracy for degraded images. This enhancement assists the T2I model in generating semantically accurate details when performing the Real-ISR task.

% Please add the following required packages to your document preamble:
% \usepackage{multirow}
\begin{table*}[h] 
\centering
\caption{Ablation study of DAPE on \textit{DIV2K-Val} and \textit{DrealSR} \cite{drealsr} benchmarks for the Real-ISR task.}
 \setlength{\tabcolsep}{1.5mm}{
\begin{tabular}{ccccccc}
\hline
\multicolumn{2}{c}{Exp}                                              & (1)           & (2)           & (3)           & (4)           & SeeSR         \\ \hline
\multirow{2}{*}{Prompt Extractor} & \multicolumn{1}{c|}{RAM \cite{2023ram}}         & \textcolor{red}{\XSolidBrush}             & \textcolor{green_c}{\Checkmark}             & \textcolor{red}{\XSolidBrush}             & \textcolor{red}{\XSolidBrush}             & \textcolor{red}{\XSolidBrush}             \\
                                  & \multicolumn{1}{c|}{DAPE}        & \textcolor{red}{\XSolidBrush}            & \textcolor{red}{\XSolidBrush}             & \textcolor{green_c}{\Checkmark}             & \textcolor{green_c}{\Checkmark}             & \textcolor{green_c}{\Checkmark}             \\ \hline
\multirow{2}{*}{Prompt Format}    & \multicolumn{1}{c|}{Hard Prompt} & \textcolor{red}{\XSolidBrush}             & \textcolor{green_c}{\Checkmark}             & \textcolor{green_c}{\Checkmark}             & \textcolor{red}{\XSolidBrush}             & \textcolor{green_c}{\Checkmark}             \\
                                  & \multicolumn{1}{c|}{Soft Prompt} & \textcolor{red}{\XSolidBrush}             & \textcolor{green_c}{\Checkmark}             & \textcolor{red}{\XSolidBrush}             & \textcolor{green_c}{\Checkmark}             & \textcolor{green_c}{\Checkmark}             \\ \hline
\multirow{4}{*}{Metrics}          & \multicolumn{1}{c|}{PSNR $\uparrow$}        & 20.96 / 27.64   & 21.15 / 27.31   & 20.91 / 27.45   & \textbf{21.19} / \textbf{28.14}   & 21.04 / 27.90   \\
                                  & \multicolumn{1}{c|}{LPIPS $\downarrow$}       & 0.4236 / 0.3130 & 0.4156 / 0.3272 & 0.4289 / 0.3285 & \textbf{0.3859} / \textbf{0.3174} & 0.3876 / 0.3299 \\
                                  & \multicolumn{1}{c|}{FID $\downarrow$}         & 37.35 / 176.26  & 46.34 / 161.69  & 38.92 / 164.57  & 38.77 / 157.63  & \textbf{32.79} / \textbf{151.88}  \\
                                  & \multicolumn{1}{c|}{CLIPIQA $\uparrow$}     & 0.6343 / 0.5693 & 0.6097 / 0.6436 & 0.6471 / 0.6410 & 0.6751 / 0.6431 & \textbf{0.6834} / \textbf{0.6708} \\ \cline{1-7} 
\end{tabular}
}
\label{lab:aba_dape}
\end{table*}

\textbf{Improved Real-ISR Performance.}
DAPE not only improves the model's ability to handle real-world degraded tags but also enhances its Real-ISR capability. We conducted a series of experiments to demonstrate the effectiveness of DAPE in Real-ISR tasks.
\begin{itemize}
  \item [1)] 
  We retrain SeeSR by removing the DAPE module and RCA module, which can be considered as applying ControlNet \cite{zhang2023adding} directly to the Real-ISR task.    
  \item [2)]
  We replace DAPE with RAM, providing hard and soft prompts, and retrain the model.
  \item [3)]
  Based on exp (1), during inference, we provide the tag text generated by DAPE as hard label input to the text encoder of the T2I model.
  \item [4)]
  During the inference of SeeSR, we remove the hard prompts.
\end{itemize}
As shown in Table \ref{lab:aba_dape}, replacing DAPE with original RAM would lead to a decrease in all perceptual metrics (\eg LPIPS and CLIPIQA). Additionally, removing the soft label would also significantly reduce both reference-based and reference-free metrics. By comparing the results of Exp. (4) with SeeSR, the introduction of hard labels can improve FID by 15\% on the \textit{DIV2K-Val} benchmark. Moreover, the visual comparisons in Fig. \ref{fig:aba_dape} also indicate inferior performance without DAPE or two kinds of prompts.

\begin{figure*}[t]
  \centering
  \includegraphics[scale=0.45]{sec/pdf/ablation_dape.png}
  \caption{Visual comparison for ablation study of DAPE. Exp. (1) does not apply RAM or DAPE, leading to blurry results. Exp. (2) applies RAM and can generate sharper details, but obvious semantically incorrect. Exp. (3) only applies hard prompts and still generates blurry results. Exp. (3) only applies soft prompts and exhibits an excessive generative capacity, leading to semantic deviations. SeeSR produces clear and semantically accurate outcomes.}

  \label{fig:aba_dape}
\end{figure*}

\begin{table}[h] 
\centering
\caption{Complexity comparison between different method. All the tests were conducted on one NVIDIA Tesla 32G-V100 GPU using public codes and their default settings, and the generated images were $512\times512$ in size.}
\begin{tabular}{c|ccc}
\hline
Methods      & \begin{tabular}[c]{@{}c} Params\end{tabular} & \begin{tabular}[c]{@{}c@{}}Inference\\ Time-steps\end{tabular} & \begin{tabular}[c]{@{}c@{}}Inference\\ Time\end{tabular} \\ \hline
Real-ESRGAN &             16.7M                                               &         1                                                       &        0.09s                                                  \\  
FeMaSR &                28.3M                                            &        1                                                        &          0.12s                                                \\
LDM         &            169.0M                                                &       200                                                         &     5.21s                                                     \\
StableSR    &       1409.1M                                                     &       200                                                         &     18.70s                                                     \\
ResShift    &      173.9M                                                      &       15                                                         &       1.12s                                                   \\
PASD        &      1900.4M                                                      &       20                                                         &     6.07s                                                     \\
DiffBIR     &      1716.7M                                                      &       50                                                         &   5.85s                                                       \\
SeeSR       &  2283.7M                                                          &       50                                                         &   7.24s                                                       \\ \hline
\end{tabular}
\label{aba: complex}
\end{table}

\section{Complexity Comparison.}
SeeSR is a diffusion-based method that requires multiple sampling to obtain SR results. As shown in Table \ref{aba: complex}, SeeSR takes 7.24s to generate a $512\times512$ image on one NVIDIA Tesla 32G-V100 GPU. This is faster than StableSR but slower than Real-ESRGAN because it only needs one forward pass. Fast sampling strategies \cite{ddim, dpm, zheng2023fast}, or model distillation \cite{meng2023distillation, salimans2022progressive} could improve the inference speed. As for the model parameters, SeeSR has 2283.7M parameters, compared to PASD and DiffBIR, the increase of model parameters mainly comes from the DAPE module, about 300M. The model parameters can be reduced by some means, such as quantization \cite{li2023q}. These explorations are beyond the scope of this paper.

\section{More Visualization Comparison.}
We provide additional qualitative comparisons on real-world images. As shown in Fig. \ref{fig:data_real_suppl}, SeeSR can generate sharper edges (case 2) and semantically faithful details (the window railing in case 1, the teeth in case 3, the vein patterns in case 4, and the feathers and eyes in case 5). Other methods are either blurry or produce unpleasant artifacts.

\begin{figure*}[t]
  \centering
  \includegraphics[scale=0.15]{sec/pdf/data_real_suppl.jpg}
  \caption{Qualitative comparisons of different methods on real-world examples. Please zoom in for a better view.}
  \label{fig:data_real_suppl}
\end{figure*}
