# Supplementary material for: SeeSR: Towards Semantics-Aware Real-World Image Super-Resolution
Source: arXiv:2311.16518 source file (2024-06-04)
Supplement: Supplementary file 2 [file suppl.tex]

\noindent
In this supplementary file, we provide the following materials:

\begin{itemize}
  \item Ablation studies on the proposed LRE strategy and DAPE module (referring to Section 4 in the main paper);
  
  \item Complexity analysis (referring to Section 4 in the main paper);
  
  \item More real-world visual comparisons under scaling factor $4\times$ (referring to Section 4.2 in the main paper).
\end{itemize}

\section{Ablation Study}
We first discuss the effectiveness of the proposed LRE strategy. Then, we discuss the effectiveness of the proposed DAPE module, including its tagging capability and the roles of hard and soft prompts.  \\

\begin{table}[b] 
\centering
\caption{The Real-ISR performance of our SeeSR model with and without LRE on \textit{DIV2K-Val} and \textit{DrealSR} \cite{drealsr} benchmarks.}
\begin{tabular}{c|cc|cc}
\hline
\multirow{2}{*}{Metrics} & \multicolumn{2}{c|}{\textit{DIV2K-Val}} & \multicolumn{2}{c}{\textit{DrealSR}} \\ \cline{2-5} 
                         & w/o LRE        & w/ LRE        & w/o LRE       & w/ LRE      \\ \hline
PSNR $\uparrow$                    & 20.58          & 21.04         & 26.55         & 27.90       \\
LPIPS   $\downarrow$                  & 0.3942         & 0.3876        & 0.3952        & 0.3299      \\
FID    $\downarrow$                   & 32.53          & 32.79         & 158.04        & 151.88      \\
CLIPIQA $\uparrow$                 & 0.7314         & 0.6834        & 0.7248        & 0.6708      \\ \hline
\end{tabular}
\label{tab: lre}
\end{table}

\noindent
\textbf{Effectiveness of LRE.} We first show the Real-ISR performance of our SeeSR model on the \textit{DIV2K-Val} and \textit{DrealSR} datasets with and without the LRE strategy. The results are shown in Table \ref{tab: lre}. One can see that the LRE strategy improves the reference-based metrics, including both fidelity and perception based ones, while it weakens the non-reference metrics such as CLIPIQA. This is because the LRE strategy reduces the model’s tendency to generate additional (but maybe unfaithful) textures by narrowing the gap between training and testing (see discussions in Section 3.4 of the main paper). Such an over-generation ability can be favorable by metrics like CLIPIQA, but they will introduce visually unpleasant artifacts, as shown in Fig. 3 of the main paper. \\

%%%%%% table aba on tag %%%%%%
\begin{table}[b] 
\centering
\caption{Comparison between RAM and DAPE on degraded images of \textit{COCO-val} benchmark \cite{coco} for the tagging task.}
\begin{tabular}{l|lll}
\hline
         & OP $\uparrow$& OR $\uparrow$ & AP $\uparrow$\\ \hline
RAM \cite{2023ram} & 0.7929   & 0.3711   &  52.3   \\
DAPE     & \textbf{0.8940}   &  \textbf{0.3751}  &  \textbf{63.0}   \\ \hline
\end{tabular}
\label{tab:aba_tag}
\end{table}
%%%%%%

\noindent
\textbf{Tagging Performance of DAPE.}
In Table \ref{tab:aba_tag}, we present the tagging performance of our DAPE module on the degraded images of \textit{COCO-val} benchmark \cite{coco} based on three metrics: overall precision (OP), overall recall (OR), and average precision (AP). AP is the averaged precision calculated on different recall rates, which is similar to the detection metric. OP and OR are defined as:
\begin{equation}
\begin{aligned}
\mathrm{OP} =\frac{\sum_{i} N_{i}^{t}}{\sum_{i} N_{i}^{p}}, && \mathrm{OR} =\frac{\sum_{i} N_{i}^{t}}{\sum_{i} N_{i}^{g}}, 
\end{aligned}
\end{equation}
where $C$ is the number of classes, $N_{i}^{p}$ is the number of images predicted for label $i$, $N_{i}^{t}$ is the number of images correctly predicted for label $i$, and $N_{i}^{g}$ is the number of ground truth images for label $i$.

We evaluate RAM \cite{2023ram} and DAPE with the default threshold. DAPE surpasses RAM in terms of OP and AP by 0.1 and 10.7, respectively. It also maintains superiority in OR, indicating that DAPE achieves significant improvements in tagging accuracy for degraded images. This improvement assists the T2I model in generating semantically accurate details when performing the Real-ISR task. \\

\begin{table*}[t]
\centering
\caption{Ablation studies of DAPE on \textit{DIV2K-Val} and \textit{DrealSR} \cite{drealsr} benchmarks for the Real-ISR task.}
 \setlength{\tabcolsep}{4mm}{
\begin{tabular}{ccccccc}
\hline
\multicolumn{2}{c}{Exp}                                              & (1)    & (2)    & (3)    & (4)    & SeeSR  \\ \hline
\multirow{2}{*}{Prompt Extractor} & \multicolumn{1}{c|}{RAM \cite{2023ram}}         & \textcolor{red}{\XSolidBrush}      & \textcolor{green_c}{\Checkmark}      & \textcolor{red}{\XSolidBrush}      & \textcolor{red}{\XSolidBrush}      & \textcolor{red}{\XSolidBrush}      \\
                                  & \multicolumn{1}{c|}{DAPE}        & \textcolor{red}{\XSolidBrush}      & \textcolor{red}{\XSolidBrush}      & \textcolor{green_c}{\Checkmark}      & \textcolor{green_c}{\Checkmark}      & \textcolor{green_c}{\Checkmark}      \\ \hline
\multirow{2}{*}{Prompt Format}    & \multicolumn{1}{c|}{Hard Prompt} & \textcolor{red}{\XSolidBrush}      & \textcolor{green_c}{\Checkmark}      & \textcolor{green_c}{\Checkmark}      & \textcolor{red}{\XSolidBrush}      & \textcolor{green_c}{\Checkmark}      \\
                                  & \multicolumn{1}{c|}{Soft Prompt} & \textcolor{red}{\XSolidBrush}      & \textcolor{green_c}{\Checkmark}      & \textcolor{red}{\XSolidBrush}      & \textcolor{green_c}{\Checkmark}      & \textcolor{green_c}{\Checkmark}      \\ \hline
\multirow{4}{*}{\textit{DIV2K-Val}}        & \multicolumn{1}{c|}{PSNR $\uparrow$}        & 20.96  & 21.15  & 20.91  & 21.19  & 21.04  \\
                                  & \multicolumn{1}{c|}{LPIPS $\downarrow$}       & 0.4236 & 0.4156 & 0.4289 & 0.3859 & 0.3876 \\
                                  & \multicolumn{1}{c|}{FID $\downarrow$}         & 37.35  & 46.34  & 38.92  & 38.77  & 32.79  \\
                                  & \multicolumn{1}{c|}{CLIPIQA $\uparrow$}     & 0.6343 & 0.6097 & 0.6471 & 0.6751 & 0.6834 \\ \hline
\multirow{4}{*}{\textit{DrealSR}}          & \multicolumn{1}{c|}{PSNR $\uparrow$}        & 27.64  & 27.31  & 27.45  & 28.14  & 27.90  \\
                                  & \multicolumn{1}{c|}{LPIPS $\downarrow$}       & 0.3130 & 0.3272 & 0.3285 & 0.3174 & 0.3299 \\
                                  & \multicolumn{1}{c|}{FID $\downarrow$}         & 176.26 & 161.69 & 164.57 & 157.63 & 151.88 \\
                                  & \multicolumn{1}{c|}{CLIPIQA $\uparrow$}     & 0.5693 & 0.6436 & 0.6410 & 0.6431 & 0.6708 \\ \hline
\end{tabular}
}
\label{lab:aba_dape}
\end{table*} 

\noindent
\textbf{Effectiveness of DAPE and Hard/Soft Prompts for Real-ISR.}
DAPE improves the model's tagging performance on degraded images and consequently enhances the Real-ISR capability. To investigate the effectiveness of DAPE and the roles of its hard/soft prompts, we conducted the following four experiments in Real-ISR tasks. \\
 
% \begin{description}[leftmargin=0.5cm, rightmargin=1cm, itemindent=0.5cm]
%   \item [Exp 1)] 
%   We retrain SeeSR by removing the DAPE and RCA modules, which can be considered as applying \\
%   ControlNet \cite{zhang2023adding} directly to the Real-ISR task.    
%   \item [Exp 2)]
%   We replace DAPE with RAM \cite{2023ram} and retrain the model.
%   \item [Exp 3)]
%  During the inference of SeeSR, we provide only the hard prompts (\ie, the tag) generated by DAPE to the text encoder of the T2I model.
%   \item [Exp 4)]
%   During the inference of SeeSR, we provide only the soft prompts (\ie, the representation embedding features) generated by DAPE to the T2I model.
% \end{description}

\begin{enumerate}[leftmargin=2em, rightmargin=2em]
  \item
  We retrain SeeSR by removing the DAPE and RCA modules, which can be considered as applying 
  ControlNet \cite{zhang2023adding} directly to the Real-ISR task.    
  \item
  We replace DAPE with RAM \cite{2023ram} and retrain the model.
  \item
 During the inference of SeeSR, we provide only the hard prompts (\ie, the tag) generated by DAPE to the text encoder of the T2I model.
  \item
  During the inference of SeeSR, we provide only the soft prompts (\ie, the representation embedding features) generated by DAPE to the T2I model.
\end{enumerate}

\begin{figure*}[t]
  \centering
  \includegraphics[scale=0.4]{sec/pdf/ablation_dape.png}
  \caption{Visual comparison for the ablation study on DAPE. Exp. (1) directly applies ControlNet to perform Real-ISR, leading to blurry results. Exp. (2) replaces DAPE with RAM for generating prompts, which can produce sharper but semantically incorrect details. Exp. (3) applies hard prompts only and generates blurry results. Exp. (4) applies soft prompts only and exhibits semantic errors in details generation. With both hard and soft prompts in DAPE, SeeSR produces clear and semantically correct outputs.}

  \label{fig:aba_dape}
\end{figure*}
\begin{figure*}[!]
  \centering
  \includegraphics[scale=0.2]{sec/pdf/data_real_suppl.jpg}
  \caption{Qualitative comparisons of different methods on real-world examples. Please zoom in for a better view.}
  \label{fig:data_real_suppl}
\end{figure*}

\vspace{3mm}
The results of the four experiments are shown in Table \ref{lab:aba_dape}. Moreover, the visual comparisons are shown in Fig. \ref{fig:aba_dape}. From Table \ref{lab:aba_dape} and Fig. \ref{fig:aba_dape}, we can have the following conclusions.

First, directly applying ControlNet to the Real-ISR task cannot achieve satisfactory results. Second, replacing DAPE with the original RAM would lead to a decrease in all perceptual metrics (\eg, LPIPS and CLIPIQA). The semantics of the image content may also be changed (see Fig. \ref{fig:aba_dape}). This is because the original RAM may generate inaccurate prompts (\eg, the tag `broccoli') from the degraded image. 
Third, the soft prompts work better in improving the numerical indices than the hard prompts, as well as sharper images. However, without hard prompts, the image semantics can be damaged, as can be seen from the lemons in Exp. (4) of Fig. \ref{fig:aba_dape}.  Finally, with both the hard and soft prompts in DAPE, perceptually realistic and semantically correct Real-ISR outputs can be produced.

\begin{table}[t] 
\centering
\caption{Complexity comparison between different methods. All the tests are conducted on one NVIDIA Tesla 32G-V100 GPU to synthesize $512\times512$ images from $128\times128$ inputs.}
\begin{tabular}{c|ccc}
\hline
Methods      & \begin{tabular}[c]{@{}c} Params\end{tabular} & \begin{tabular}[c]{@{}c@{}}Inference\\ Time-steps\end{tabular} & \begin{tabular}[c]{@{}c@{}}Inference\\ Time\end{tabular} \\ \hline
Real-ESRGAN \cite{wang2021real} &             16.7M                                               &         1                                                       &        0.09s                                                  \\  
FeMaSR \cite{chen2022femasr}&                28.3M                                            &        1                                                        &          0.12s                                                \\
LDM  \cite{rombach2022high}       &            169.0M                                                &       200                                                         &     5.21s                                                     \\
StableSR \cite{wang2023exploiting}   &       1409.1M                                                     &       200                                                         &     18.70s                                                     \\
ResShift  \cite{yue2023resshift}  &      173.9M                                                      &       15                                                         &       1.12s                                                   \\
PASD    \cite{yang2023pixel}    &      1900.4M                                                      &       20                                                         &     6.07s                                                     \\
DiffBIR  \cite{lin2023diffbir}   &      1716.7M                                                      &       50                                                         &   5.85s                                                       \\
SeeSR       &  2283.7M                                                          &       50                                                         &   7.24s                                                       \\ \hline
\end{tabular}
\label{aba: complex}
\end{table}

\section{Complexity Analysis}
Table \ref{aba: complex} compares the number of parameters of different Real-ISR models and their inference time to synthesize a $512\times512$ image from $128\times128$ input. All tests are conducted on one NVIDIA Tesla 32G-V100 GPU. We can have the following observations.

First, the GAN-based methods Real-ESRGAN and FeMaSR have much less model parameters and much faster inference speed than DM-based methods. Second, among the DM-based models, LDM and ResShift are much smaller than others because they employ relatively lightweight diffusion models. ResShift runs faster than LDM because it samples only 15 steps while LDM samples 200 steps. Thrid, StableSR, PASD, DiffBIR and our SeeSR are all based on the pre-trained T2I model. SeeSR has more parameters because it has a DAPE module (about 300M) finetuned from the RAM model. In terms of inference speed, PASD, DiffBIR and SeeSR are comparable, while StableSR is the slowest one because it samples 200 steps.   

%SeeSR is a diffusion-based method that requires multiple sampling to obtain SR results. As shown in Table \ref{aba: complex}, SeeSR takes 7.24s to generate a $512\times512$ image on one NVIDIA Tesla 32G-V100 GPU. This is faster than StableSR but slower than Real-ESRGAN because it only needs one forward pass. Fast sampling strategies \cite{ddim, lu2022dpm, zheng2023fast}, or model distillation \cite{meng2023distillation, salimans2022progressive} could improve the inference speed. As for the model parameters, SeeSR has 2283.7M parameters, compared to PASD and DiffBIR, the increase of model parameters mainly comes from the DAPE module, about 300M. The model parameters can be reduced by some means, such as quantization \cite{li2023q}. These explorations are beyond the scope of this paper.

% \section{More Visualization Comparisons}
% We provide additional qualitative comparisons on real-world images. As shown in Fig. \ref{fig:data_real_suppl}, SeeSR can generate sharper edges (case 2) and semantically faithful details (the window railing in case 1, the teeth in case 3, and the vein textures in case 4). Other methods are either blurry or produce unpleasant artifacts.

\vfill
